# Supplementary material for: Overcoming Reward Overoptimization via Adversarial Policy Optimization with Lightweight Uncertainty Estimation
Source: arXiv:2403.05171 source file (2024-07-09)
Supplement: Supplementary file 1 [file appendix_exp.tex]

\section{Additional Experiments}

\subsection{Effect of number of ensembles.}
\label{appendix-subsec-ens-3b-5}
We chose to use three ensembles to compare our methods with ensemble-based uncertainty quantification approaches of comparable size. We opted for three ensembles as our approach utilized Llama 7B, and the smallest available Llama model is OpenLLaMA3B. OpenLLaMA is an open-source reproduction of Meta AI’s LLaMA, which demonstrates comparable performance.

To analyze the impact of the number of ensembles, we extend our analysis to include a configuration with 5 ensembles, denoted as ENS-3B-5.
Figures \ref{fig:hh-step-3b-5} and \ref{fig:tldr-step-3b-5} display the results.
As observed from Figure \ref{fig:tldr-step-3b-5}, even with five ensembles, ENS-3B-5 does not consistently demonstrate an increasing trend in the reward difference between gold and proxy rewards in the TLDR dataset, indicating its deficiency in accurately capturing reward uncertainty. This suggests that perhaps the size of the reward model is more crucial than the number of ensembles.
\begin{figure*}[t]
  \centering
  % % \vspace{-2mm}
  \subfloat[Anthropic HH with ENS-3B-5]
           { \includegraphics[width=0.45\linewidth, height=.4\linewidth]{paper/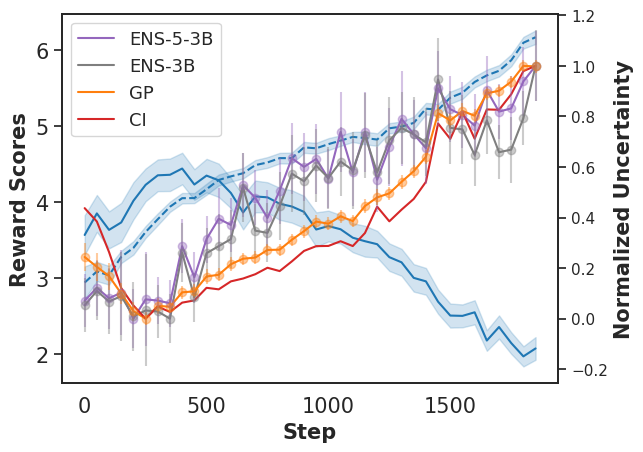}
             \label{fig:hh-step-3b-5}}
  \subfloat[TLDR with ENS-3B-5]
           { \includegraphics[width=0.45\linewidth, height=.4\linewidth]{paper/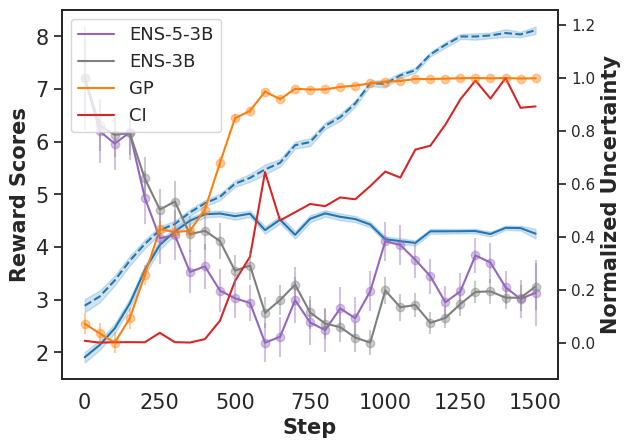}
             \label{fig:tldr-step-3b-5}}
 \caption{Comparison among lightweight uncertainty estimations with ENS-3B-5. The blue lines with shaded areas depict the reward
dynamics concerning optimization steps in PPO, where the solid and dashed lines represent gold and proxy rewards, respectively. The
lines with dots denote the results from different uncertainty estimation methods. The reward values are indexed on the left y-axis, while
the uncertainty is indexed on the right y-axis.
}
    \label{fig:overopt}
% \vspace{-4mm}
\end{figure*}

\subsection{\model{} can address overoptimization: A second pespective. }
In Figure \ref{fig:hh-advpo-un-ppo} and \ref{fig:tldr-advpo-un-ppo}, we plot  the evolution of the average uncertainty of generated responses by PPO and \model{} across optimization steps for experiments in Section \ref{subsec:overopt}. 
And Figure \ref{fig:hh-advpo-un-pen} and Figure \ref{fig:tldr-advpo-un-pen} depict the average uncertainty penalization of \model{} over optimization steps.
We can observe from Figure \ref{fig:hh-advpo-un-ppo} and \ref{fig:tldr-advpo-un-ppo} that the average uncertainties of generated responses remain stable under \model, in contrast to the significant increase in uncertainty observed with PPO.

\begin{figure*}[th]
  \centering
  % % \vspace{-2mm}
  \subfloat[Anthropic HH (UN)]
           { \includegraphics[width=.25\linewidth, height=.18\linewidth]{paper/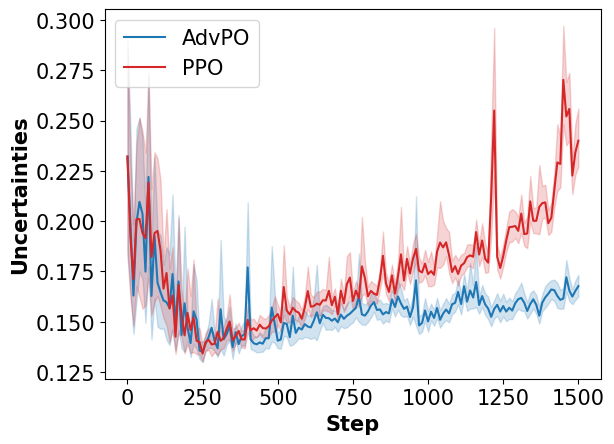}
             \label{fig:hh-advpo-un-ppo}}
  \subfloat[Anthropic HH (UN Penalty)]
           { \includegraphics[width=.25\linewidth, height=.18\linewidth]{paper/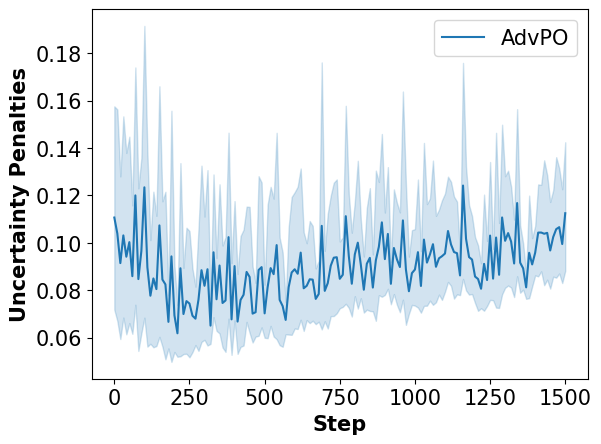}
             \label{fig:hh-advpo-un-pen}}
  \subfloat[TL;DR (UN)]
           { \includegraphics[width=.25\linewidth, height=.18\linewidth]{paper/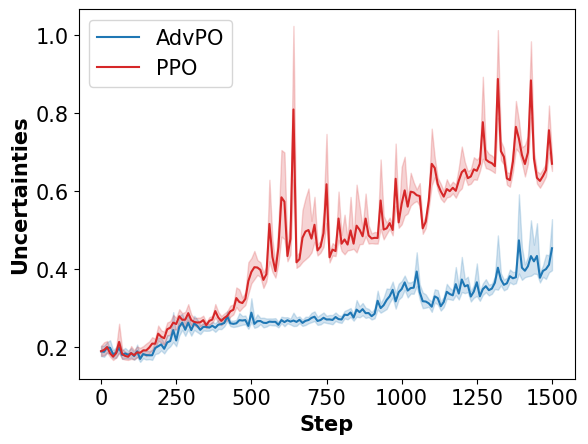}
             \label{fig:tldr-advpo-un-ppo}}
  \subfloat[TL;DR (UN Penalty)]
           { \includegraphics[width=.25\linewidth, height=.18\linewidth]{paper/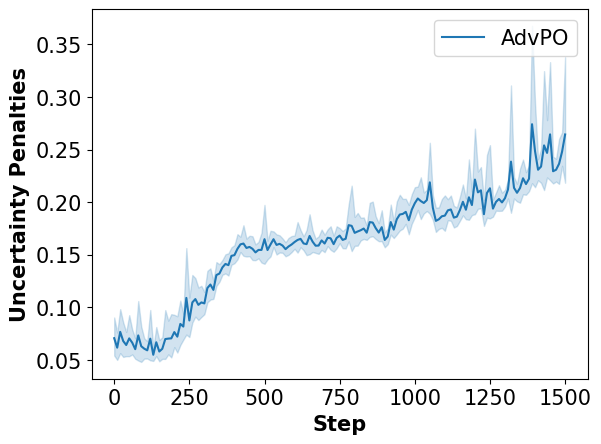}
             \label{fig:tldr-advpo-un-pen}}
 % % \vspace{0}
    \caption{ Another perspective  of how \model addresses overoptimization.
    }
    \label{fig:overopt}
% \vspace{-4mm}
\end{figure*}
